# Supplementary material for: Relationship between crystal structure and multiferroic orders in orthorhombic perovskite manganites
Source: arXiv:1805.02172 ancillary file (2018-06-08)
Supplement: Supplementary file 1 [file supplemental.pdf]

# Relationship between crystal structure and multiferroic orders in orthorhombic perovskite manganites
# - Supplemental Materials -

Natalya S. Fedorova,[1,*] Yoav William Windsor,[2] Christoph Findler,[1] Mahesh Ramakrishnan,[2] Amadé Bortis,[3] Laurenz Rettig,[2] Kenta Shimamoto,[4] Elisabeth M. Bothschafter,[2] Michael Porer,[2] Vincent Esposito,[2] Yi Hu,[4] Aurora Alberca,[2] Thomas Lippert,[4,5] Christof W. Schneider,[4] Urs Staub,[2] and Nicola A. Spaldin[1,†]

[1]*Materials Theory, ETH Zürich, Wolfgang-Pauli-Strasse 27, CH-8093 Zürich, Switzerland*
[2]*Swiss Light Source, Paul Scherrer Institut, CH-5232 Villigen PSI, Switzerland*
[3]*Laboratory for Multifunctional Ferroic Materials, ETH Zürich, Vladimir-Prelog-Weg 4, CH-8093 Zürich, Switzerland*
[4]*Laboratory for Multiscale Materials Experiments, Paul Scherrer Institut, CH-5232 Villigen PSI, Switzerland*
[5]*Laboratory of Inorganic Chemistry, Department of Chemistry and Applied Biosciences, ETH Zürich, CH-8093, Zürich, Switzerland*

## I. CRYSTAL STRUCTURES

Table I present a list of all crystalline films indicated in the experimental section (Sec. III of the main text). The last entries are values taken from literature. Error estimates of $q_b$ values are smaller than the last digit. All substrates were $YAlO_3$ unless otherwise indicated. The incommensurate modulation $q_b$ varies with temperature. $q_b$ values here are given at the experimental base temperature of 10 K.

In Table II we summarize experimentally reported (Refs. 5–10) and theoretically optimized lattice parameters of bulk o-$R$MnO$_3$ ($R$=Gd, Tb, Ho, Er, Yb, Lu), which were discussed in Sec. V of the main text. Table III shows the experimentally measured (Refs. 3 and 4 and our measurements) and theoretically optimized lattice parameters of the corresponding strained films (see Sec. V of the main text). We provide .cif files for all theoretically optimized structures in Supplemental materials.

Table I. Experimentally acquired parameters of epitaxial o-$R$MnO$_3$ films. Thickness ($t$) and substrate normal ($n$) are controlled growth parameters. $q_b$ is deduced from RXD experiments at the Mn $L$ edges. Error estimates of $q_b$ values are smaller than the last digit (unless otherwise indicated). Lattice constants were deduced in conventional XRD experiments.

| $R$ | $t$ (nm) | $n$ | $q_b$ | $a$ (Å) | $b$ (Å) | $c$ (Å) | Comment |
|---|---|---|---|---|---|---|---|
| Yb | 400 | [010] | 0.4747 | 5.223 ± 0.004 | 5.771 ± 0.007 | 7.361 ± 0.008 | |
| Er | 400 | [010] | 0.4496 | 5.235 ± 0.002 | 5.799 ± 0.002 | 7.359 ± 0.002 | |
| Er | 30 | [010] | 0.5015 | 5.1735 ± 0.0005 | 5.828 ± 0.001 | 7.360 ± 0.001 | |
| Ho | 240 | [010] | 0.4007 ± 0.0001 | 5.275 ± 0.001 | 5.789 ± 0.005 | 7.392 ± 0.001 | Grown on $NdGaO_3$ |
| Ho | 120 | [010] | 0.4138 ± 0.0002 | 5.2748 ± 0.0007 | 5.779 ± 0.005 | 5.420 ± 0.004 | Grown on $NdGaO_3$ |
| Tm | 400 | [010] | 0.4625 | 5.235 ± 0.001 | 5.779 ± 0.001 | 7.3737 ± 0.0008 | Windsor *et al.*[1] |
| Tm | 56 | [110] | 0.4704 ± 0.0001 | 5.221 ± 0.001 | 5.757 ± 0.004 | 7.342 ± 0.005 | |
| Lu | 104 | [010] | 0.4861 | 5.2200 ± 0.0001 | 5.753 ± 0.005 | 7.3797 ± 0.0008 | |
| Lu | 400 | [110] | 0.4956 | 5.191 ± 0.002 | 5.760 ± 0.004 | 7.365 ± 0.004 | |
| Lu | 90 | [110] | 0.4933 ± 0.0001 | 5.175 ± 0.002 | 5.717 ± 0.001 | 7.370 ± 0.002 | |
| Lu | 78 | [010] | 0.4857 | 5.230 ± 0.005 | 5.766 ± 0.005 | 7.380 ± 0.007 | |
| Lu | 26 | [010] | 0.4797 | 5.220 ± 0.005 | 5.734 ± 0.005 | 7.492 ± 0.007 | |
| Tb | 10 | [010] | 0.4539 ± 0.0001 | 5.259 ± 0.001 | 5.801 ± 0.001 | 7.355 ± 0.001 | |
| Tb | 200 | [010] | 0.2619 ± 0.0001 | / | 5.8014 ± 0.0001 | / | |
| Y | 40 | [010] | 0.491 | ?? | ?? | ?? | Wadati *et al.*[2] |
| Tb | 14 | [010] | 0.5 | 5.182 | 5.936 | 7.367 | Shimamoto *et al.*[3] |
| Gd | 10 | [010] | 0.5 | 5.183 | 5.976 | 7.372 | Shimamoto *et al.*[4] |

Table II. Experimentally reported (Exp.) and theoretically optimized (PS) lattice parameters of bulk o-$R$MnO$_3$. $a$, $b$ and $c$ are the lattice constants of $Pbnm$ (#62) orthorhombic unit cell; $s$, $m$ and $l$ denote short, medium and long Mn-O bonds of MnO$_6$ octahedra; $d_O$ is the distance between oxygens O(1) and O(2) shown in Fig. 1(b) of the main text; IPA and OPA are the Mn-O-Mn bond angles within the $ab$ planes and along the $c$ direction, respectively. All the lengths are in Å and all the angles are in degrees.

| | GdMnO$_3$ | | TbMnO$_3$ | | HoMnO$_3$ | | ErMnO$_3$ | | YbMnO$_3$ | | LuMnO$_3$ | |
|---|---|---|---|---|---|---|---|---|---|---|---|---|
| | Exp.[5] | PS | Exp.[6] | PS | Exp.[7] | PS | Exp.[8] | PS | Exp.[9] | PS | Exp.[10] | PS |
| $a$ | 5.318 | 5.261 | 5.293 | 5.240 | 5.257 | 5.203 | 5.227 | 5.186 | 5.216 | 5.154 | 5.190 | 5.137 |
| $b$ | 5.866 | 5.807 | 5.838 | 5.797 | 5.835 | 5.771 | 5.792 | 5.759 | 5.799 | 5.725 | 5.785 | 5.706 |
| $c$ | 7.431 | 7.367 | 7.403 | 7.342 | 7.361 | 7.301 | 7.327 | 7.282 | 7.299 | 7.253 | 7.282 | 7.241 |
| $s$ | 1.911 | 1.916 | 1.905 | 1.915 | 1.904 | 1.912 | 1.910 | 1.911 | 1.879 | 1.908 | 1.899 | 1.907 |
| $m$ | 1.944 | 1.934 | 1.940 | 1.934 | 1.944 | 1.936 | 1.938 | 1.936 | 1.940 | 1.940 | 1.942 | 1.942 |
| $l$ | 2.228 | 2.182 | 2.221 | 2.180 | 2.223 | 2.173 | 2.194 | 2.170 | 2.262 | 2.160 | 2.206 | 2.155 |
| $l_{O-O}$ | 3.097 | 3.071 | 3.057 | 3.047 | 3.020 | 3.007 | 2.993 | 2.990 | 2.907 | 2.959 | 2.967 | 2.945 |
| IPA | 145.98 | 145.80 | 145.36 | 145.08 | 144.08 | 143.85 | 143.66 | 143.32 | 140.51 | 142.32 | 142.26 | 141.81 |
| OPA | 145.68 | 145.38 | 145.04 | 143.19 | 142.46 | 141.08 | 141.91 | 140.15 | 140.27 | 138.40 | 139.30 | 137.51 |

Table III. Experimentally measured and theoretically optimized lattice parameters of films of o-$R$MnO$_3$. $a$, $b$ and $c$ are the lattice constants of $Pbnm$ (#62) orthorhombic unit cell; $s$, $m$ and $l$ denote short, medium and long bonds of MnO$_6$ octahedra; $d_O$ is a distance between oxygens O(1) and O(2) shown in Fig. 1(b) of the main text; IPA and OPA are the Mn-O-Mn bond angles within the $ab$ planes and along the $c$ direction, respectively. All the lengths are in Å and all the angles are in degrees.

| | GdMnO$_3$ | | TbMnO$_3$ | | HoMnO$_3$ | | ErMnO$_3$ | | YbMnO$_3$ | | LuMnO$_3$ | | | |
|---|---|---|---|---|---|---|---|---|---|---|---|---|---|---|
| | 10 nm | | 14 nm | | 120 nm | | 30 nm | | 400 nm | | 26 nm | | 104 nm | |
| | Exp.[4] | PS | Exp.[3] | PS | Exp. | PS | Exp. | PS | Exp. | PS | Exp. | PS | Exp. | PS |
| $a$ | 5.183 | 5.128 | 5.182 | 5.130 | 5.275 | 5.220 | 5.174 | 5.132 | 5.224 | 5.161 | 5.220 | 5.167 | 5.220 | 5.167 |
| $b$ | 5.976 | 5.935 | 5.936 | 5.893 | 5.780 | 5.736 | 5.828 | 5.780 | 5.771 | 5.699 | 5.734 | 5.595 | 5.753 | 5.651 |
| $c$ | 7.372 | 7.309 | 7.367 | 7.307 | 7.429 | 7.368 | 7.360 | 7.315 | 7.361 | 7.315 | 7.492 | 7.450 | 7.379 | 7.338 |
| $s$ | - | 1.909 | - | 1.909 | - | 1.914 | - | 1.908 | - | 1.909 | - | 1.910 | - | 1.909 |
| $m$ | - | 1.915 | - | 1.921 | - | 1.951 | - | 1.940 | - | 1.953 | - | 1.990 | - | 1.965 |
| $l$ | - | 2.204 | - | 2.195 | - | 2.164 | - | 2.167 | - | 2.153 | - | 2.120 | - | 2.141 |
| $l_{O-O}$ | - | 3.000 | - | 2.990 | - | 3.025 | - | 2.970 | - | 2.973 | - | 3.008 | - | 2.978 |
| IPA | - | 144.81 | - | 144.30 | - | 143.89 | - | 142.95 | - | 142.27 | - | 141.75 | - | 141.85 |
| OPA | - | 145.09 | - | 143.88 | - | 141.50 | - | 140.93 | - | 138.85 | - | 138.72 | - | 138.02 |

## II. EXCHANGE INTERACTIONS AND ANISOTROPIES

In Tables IV and V we summarize the Heisenberg ($J_c$, $J_{ab}$, $J_a$, $J_{diag}$, $J_b$ and $J_{3nn}$), biquadratic ($B_c$ and $B_{ab}$) and four-spin ring ($K_c$ and $K_{ab}$) exchange interactions as well as the Dzyaloshinskii-Moriya interaction (DMI, $\gamma_{ab}$ and $\alpha_c$) and single ion anisotropy ($A$) parameters calculated using DFT for bulk samples and films of o-$R$MnO$_3$, respectively.

In Fig. 1 we present the calculated couplings $J_a$, $J_{diag}$, $B_c$, $K_{ab}$, $\gamma_{ab}$ and $\alpha_c$ and anisotropies A versus the radius of the $R$ cations for the bulk and film geometries.


* natalya.fedorova@mat.ethz.ch
† nicola.spaldin@mat.ethz.ch


1 Y. W. Windsor, M. Ramakrishnan, L. Rettig, A. Alberca, E. M. Bothschafter, U. Staub, K. Shimamoto, Y. Hu, T. Lippert, and C. W. Schneider, Phys. Rev. B **91**, 235144 (2015).
2 H. Wadati, J. Okamoto, M. Garganourakis, V. Scagnoli, U. Staub, Y. Yamasaki, H. Nakao, Y. Murakami, M. Mochizuki, M. Nakamura, et al., Phys. Rev. Lett. **108**, 047203 (2012).

Table IV. Heisenberg ($J_c$, $J_{ab}$, $J_a$, $J_{diag}$, $J_b$, $J_{3nn}$), four-spin ring ($K_{ab}$ and $K_c$) and biquadratic ($B_{ab}$ and $B_c$) exchanges, components of DM vectors ($\gamma_{ab}$ and $\alpha_c$) and single-ion anisotropies ($A$) (in meV) calculated using DFT for bulk o-$R$MnO$_3$.

| $R$ | $J_c$ | $J_{ab}$ | $J_a$ | $J_{diag}$ | $J_b$ | $J_{3nn}$ | $K_{ab}$ | $K_c$ | $B_{ab}$ | $B_c$ | $\gamma_{ab}$ | $\alpha_c$ | $A$ |
|---|---|---|---|---|---|---|---|---|---|---|---|---|---|
| Gd | 4.34 | -7.04 | -0.99 | 0.75 | 0.67 | 2.82 | 0.24 | 0.91 | -2.25 | -0.44 | -0.57 | -0.50 | -0.47 |
| Tb | 4.35 | -6.03 | -0.96 | 0.73 | 0.76 | 2.75 | 0.23 | 0.90 | -2.20 | -0.43 | -0.57 | -0.47 | -0.48 |
| Ho | 4.33 | -4.44 | -0.95 | 0.72 | 0.95 | 2.69 | 0.21 | 0.92 | -1.75 | -0.42 | -0.57 | -0.42 | -0.48 |
| Er | 4.20 | -3.81 | -0.99 | 0.69 | 0.95 | 2.68 | 0.28 | 0.90 | -2.25 | -0.45 | -0.58 | -0.40 | -0.49 |
| Yb | 4.03 | -2.73 | -0.96 | 0.68 | 1.07 | 2.68 | 0.28 | 0.94 | -2.22 | -1.13 | -0.58 | -0.37 | -0.48 |
| Lu | 3.96 | -2.20 | -0.94 | 0.68 | 1.13 | 2.70 | 0.28 | 0.96 | -2.29 | -0.88 | -0.61 | -0.35 | -0.47 |

Table V. Heisenberg ($J_c$, $J_{ab}$, $J_a$, $J_{diag}$, $J_b$, $J_{3nn}$), four-spin ring ($K_{ab}$ and $K_c$) and biquadratic ($B_{ab}$ and $B_c$) exchanges, components of DM vectors ($\gamma_{ab}$ and $\alpha_c$) and single-ion anisotropies ($A$) (in meV) calculated using DFT for the films of o-$R$MnO$_3$. Lu$^{(1)}$ correspond to 104 nm film, Lu$^{(2)}$ - 26 nm film, Lu$^{(3)}$ - inv104 case, Lu$^{(4)}$ - inv26 case.

| $R$ | $J_c$ | $J_{ab}$ | $J_a$ | $J_{diag}$ | $J_b$ | $J_{3nn}$ | $K_{ab}$ | $K_c$ | $B_{ab}$ | $B_c$ | $\gamma_{ab}$ | $\alpha_c$ | $A$ |
|---|---|---|---|---|---|---|---|---|---|---|---|---|---|
| Gd | 7.80 | -1.27 | -0.82 | 0.70 | 1.02 | 2.22 | 0.20 | 0.71 | -1.82 | 0.43 | -0.51 | -0.42 | -0.52 |
| Tb | 4.35 | -6.03 | -0.96 | 0.73 | 0.76 | 2.75 | 0.23 | 0.90 | -2.20 | -0.43 | -0.57 | -0.47 | -0.48 |
| Ho | 2.60 | -6.51 | -1.00 | 0.72 | 0.79 | 2.90 | 0.21 | 0.99 | -2.33 | -1.21 | -0.63 | -0.51 | -0.44 |
| Er | 4.18 | -2.79 | -0.97 | 0.69 | 1.02 | 2.61 | 0.27 | 0.90 | -2.23 | -0.62 | -0.60 | -0.44 | -0.47 |
| Yb | 2.88 | -4.29 | -1.02 | 0.69 | 0.95 | 2.85 | 0.29 | 1.01 | -2.39 | -0.54 | -0.63 | -0.45 | -0.44 |
| Lu$^{(1)}$ | 1.98 | -5.48 | -1.10 | 0.68 | 0.87 | 3.04 | 0.33 | 1.08 | -2.65 | -2.16 | -0.70 | -0.48 | -0.41 |
| Lu$^{(2)}$ | 0.14 | -8.68 | -1.16 | 0.78 | 0.85 | 3.48 | 0.12 | 1.32 | -2.52 | -4.71 | -0.96 | -0.69 | -0.33 |
| Lu$^{(3)}$ | 5.85 | 1.23 | -0.82 | 0.71 | 1.37 | 2.31 | 0.25 | 0.83 | -1.74 | 0.31 | -0.52 | -0.23 | -0.52 |
| Lu$^{(4)}$ | 6.67 | 3.22 | -0.78 | 0.65 | 2.16 | 1.46 | 0.77 | 0.67 | -2.65 | 0.07 | -0.44 | -0.09 | -0.57 |


[3] K. Shimamoto, S. Mukherjee, S. Manz, J. S. White, M. Trassin, M. Kenzelmann, L. Chapon, T. Lippert, M. Fiebig, C. W. Schneider, et al., Scientific Reports **7**, 44753 (2017).

[4] K. Shimamoto, S. Mukherjee, N. S. Bingham, A. K. Suszka, T. Lippert, C. Niedermayer, and C. W. Schneider, Phys. Rev. B **95**, 184105 (2017).

[5] T. Mori, N. Kamegashira, K. Aoki, T. Shishido, and T. Fukuda, Materials Lett. **54**, 238 (2002), ISSN 0167-577X.

[6] J. A. Alonso, M. J. Martínez-Lope, M. T. Casáis, and M. T. Fernandez-Díaz, Inorg. Chem. **39**, 917 (2000).

[7] A. Muñoz, M. T. Casáis, J. A. Alonso, M. J. Martínez-Lope, J. L. Martínez, and M. T. Fernández-Díaz, Inorg. Chem. **40**, 1020 (2001).

[8] F. Ye, B. Lorenz, Q. Huang, Y. Q. Wang, Y. Y. Sun, C. W. Chu, J. A. Fernandez-Baca, P. Dai, and H. A. Mook, Physical Review B **76**, 060402 (2007).

[9] M. Tachibana, T. Shimoyama, H. Kawaji, T. Atake, and E. Takayama-Muromachi, Phys. Rev. B **75**, 144425 (2007).

[10] H. Okamoto, N. Imamura, B. Hauback, M. Karppinen, H. Yamauchi, and H. Fjellvåg, Solid State Comm. **146**, 152 (2008).

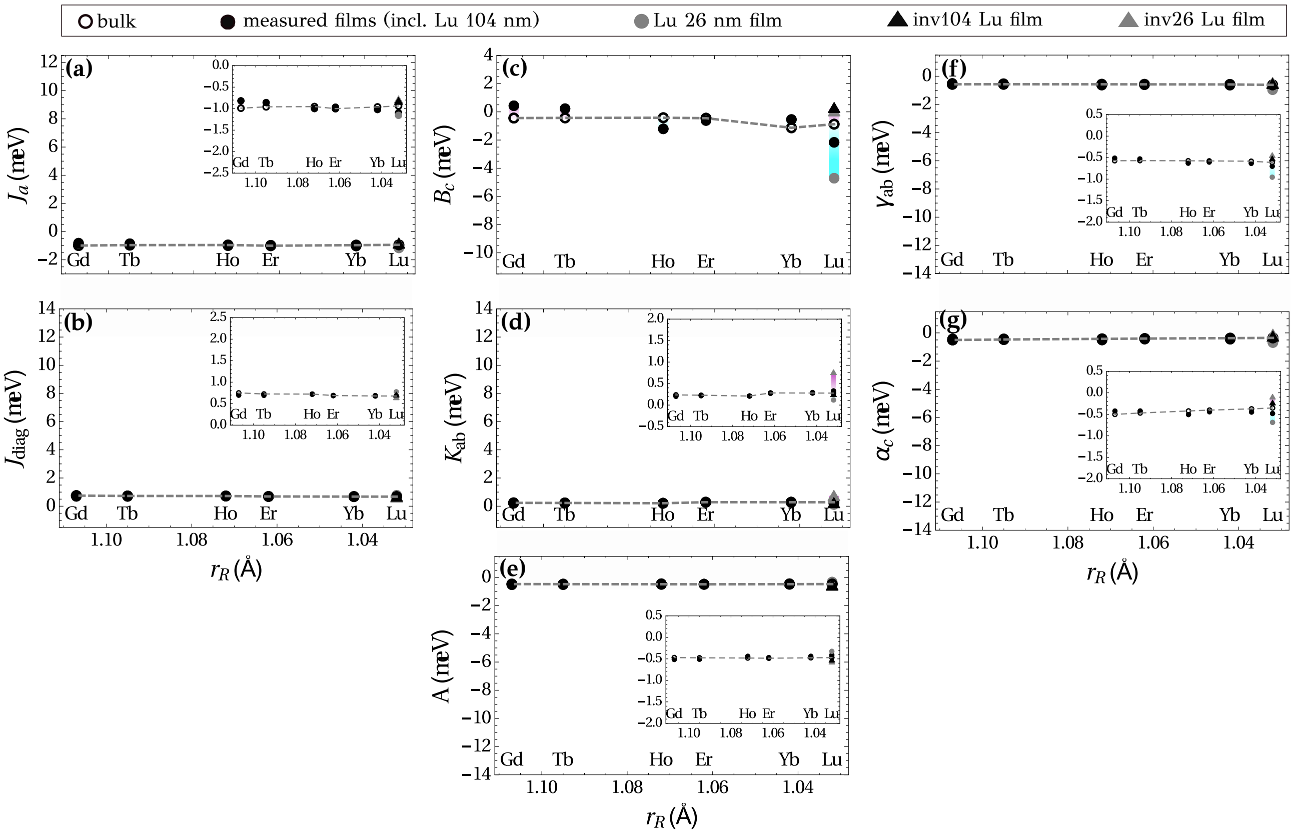


Figure 1. Calculated exchange couplings, components of DM vectors and anisotropy constants versus the radius of the $R$ cation: (a) and (b) show the Heisenberg exchanges $J_a$ and $J_{diag}$, respectively; (c) - biquadratic interplane exchanges $B_c$; (d) - four-spin ring couplings $K_{ab}$; (e) - SIA $A$; (f) and (g) - the components of DM vectors $\gamma_{ab}$ and $\alpha_c$, respectively. Bulk samples are shown by the empty circles, experimentally measured strained films - by the filled circles. In most cases filled and empty circles are on top of each other. For $LuMnO_3$ the triangles denote the films which are compressively strained in the $ac$ plane by the same amount (but opposite direction) as experimentally measured tensily strained films. $LuMnO_3$ 26 nm film and corresponding inverse case are highlighted in gray, 104 nm and inv104 case - in black. Compressive strain within the $ac$ planes of the o-$R$MnO$_3$ films shown by the violet color, tensile strain - by the blue color. Dashed line connecting the data points for the bulk o-$R$MnO$_3$ is used to guide eye.
